# Supplementary material for: A Safe Reinforcement Learning Algorithm for Supervisory Control of Power Plants
Source: arXiv:2401.13020 source file (2024-01-23)
Supplement: Supplementary file 1 [file additional_text.tex]

\begin{comment}
One of the primary challenges faced in reinforcement learning is the design of a proper reward function which can efficiently guide the learning process. Many real world problems are multi-objective problems in which conflicting objectives should be optimized. A common approach to handling multi-objective problems in RL is to combine the objectives using a set of coefficients \cite{mannor2004geometric}. With this approach, there exist a set of optimal solutions for each set of coefficients, known as the Pareto optimal solutions \cite{van2014multi}. In practice, finding the set of coefficients which leads to the desired solutions is not a trivial task. For many problems, it is more natural to specify a single objective and a set of constraints. The CMDP framework is the standard formulation for RL problems involving constraints \cite{altman1999constrained}. Optimal policies for CMDPs can be obtained by solving an equivalent linear programming formulation \cite{altman1999constrained}, or via multi time-scale dynamic-programming based algorithms  \cite{bhatnagar2012online,bhatnagar2010actor,borkar2005actor,geibel2012learning,geibel2005risk}. Such methods may not be applicable to large scale problems or problems with continuous state-action space. Leveraging recent advances in deep learning and policy search methods \cite{schulman2015trust}, some works devise multi-time scale algorithms for solving RL problems in presence of constraints \cite{tessler2018reward,liang2018accelerated,fu2018risk,chow2017risk, achiam2017constrained}. Broadly speaking, these methods are either based on Lagrangian relaxation \cite{tessler2018reward,liang2018accelerated,fu2018risk,chow2017risk} or constrained policy optimization \cite{achiam2017constrained}. In Lagrangian relaxtion based method, primal and dual variables are updated at different time-scales using gradient ascent/descent. In these methods, constraint satisfaction is guaranteed at convergence. On the other hand, in \cite{achiam2017constrained} an algorithm is proposed where constraint satisfaction is enforced in every step throughout training. 
\end{comment}

\begin{comment}
\begin{itemize}
    \item RL environment for solving optimization and control tasks in Modelica models \cite{lukianykhin2019modelicagym}.
    
    \item Comparison of RL (fitted Q-iterations)with MPC applied to a deterministic electrical power oscillations damping problem \cite{ernst2008reinforcement}.
    
    \item Closed-loop control of (dis)charging rate of a thermal storage tank using Q-learning \cite{henze2003evaluation}.
    
    \item Control of heating ventilation and air conditioning
(HVAC) heating system with PPO \cite{wang2018novel}.

    \item RL-based dispatch of combined Heat and Power (CHP) systems using distributed PPO \cite{zhou2020combined}.
\end{itemize}
\end{comment}


\begin{comment}
\begin{algorithm} \label{Alg1}
 \SetKwInOut{Input}{Input}
    \LinesNotNumbered
    \Input{Initial policy network parameters $\vect{\theta}$, initial value network parameters $\vect{\Theta}$, initial Lagrange multipliers $\vect{\eta}=\vect{0}$  }
\For{$\text{epoch}=0,1, \cdots$ }
{
\For{$n=0,1, \cdots$, $H$}
{
Observe initial state $s_n$ \\
Sample action $a_n \sim \pi_{\vect{\theta}}(a_n|s_n)$\\
Take action $a_n$\\
Receive reward $\mathcal{R}(s_n,a_n)$, $M$ costs $\mathcal{C}_m(s_n,a_n)$, and new state $s_{n+1}$\\
Compute penalized reward $\hat{\mathcal{R}}(s_n,a_n,\vect{\eta})$ using \eqref{pen:rew} \\
Store transition $(s_n,a_n,\hat{\mathcal{R}}(s_n,a_n,\vect{\eta}),s_{n+1})$ in policy training buffer\\
Store $\mathcal{C}_{k,\forall k}(s_n,a_n)$ in Lagrange multiplier training buffer
}
Compute rewards to go\\
Compute advantage estimate $\hat{A}_n$ using GAE \eqref{gae} and current value network\\
\For{$k=0,1,\cdots$}
{
Update policy parameters ${\vect{\theta}}_k$ via stochastic gradient ascent with ADAM on the PPO-Clip objective \eqref{ppo} \\
Compute KL-divergence between new policy and old policy\\
Break if KL-divergence hits $\text{KL}_{\text{Th}}$\\
}
\For{$k=0,1,\cdots$}
{
Fit the value network via stochastic gradient descent with ADAM on \eqref{mse:V}
}
Update Lagrangian multipliers via stochastic gradient descent with ADAM on  \eqref{lag:loss}
}
    \caption{Constrained PPO-Clip}
\end{algorithm}

To parameterize the space of continuous control policies, a parameterized stochastic Gaussian policy is adopted \cite{sutton2018reinforcement},
\begin{equation}
    \pi_{\vect{\theta}} (a_n|s_n) = \frac{1}{\sigma(s_n,\vect{\theta_\sigma})\sqrt{2\pi}} \text{exp} \Big(- \frac{(a_n - \mu(s_n,\vect{\theta_\mu}))^2}{2\sigma(s_n,\vect{\theta_\sigma})^2} \Big).
\end{equation}
where $\vect{\theta_\mu}$ are the DNN parameters for the mean of the policy, and $\vect{\theta_\sigma}$ are the DNN parameters for the variance of the policy. The choice of a gaussian policy is commonly adopted in DRL because the gradient of the policy as well as the log probabilities necessary for KL-divergence computation can be derived in a closed form \cite{sutton2018reinforcement}. At the beginning of training, the variance of the policy network encourages exploration. As training progresses, the variance of the policy is reduced due to maximizing \eqref{ppo} and in doing so, the policy shifts slowly towards the deterministic policy given by $\mu(s_n,\vect{\theta_\mu})$.
\end{comment}


\begin{comment}

\subsubsection{Soft Actor-Critic (SAC)}

SAC  is a state-of-the-art off-policy RL algorithm which is based on the maximum entropy RL framework. SAC exhibits high sample efficiency by reusing historical samples, does not require sensitive hyperparameter tuning thanks to the entropy term in the training objective, and produces smooth actions by temporally correlating exploration. In SAC, the RL agent receives an extra reward that is the entropy of the policy $\mathcal{H}(\pi_{\vect{\theta}}(a_t|s_t)) =\mathbb{E}_{a_{t} }[-\text{log}~\pi_{\vect{\theta}}(a_t|s_{t})]$, %we can add the entropy bonus during simulation because of the expectation over s_{t+1}
\begin{equation}
\begin{aligned}
    \mathcal{R}^{\text{SAC}}&(s_t,a_t) = \mathcal{R}(s_t,a_t) + \alpha\mathbb{E}_{s_{t+1} \sim \mathcal{P}} [\mathcal{H}(\pi_{\vect{\theta}}(.|s_{t+1})]
    \\
    &= \mathcal{R}(s_t,a_t) + \alpha \mathbb{E}_{s_{t+1} \sim \mathcal{P}} \big[\mathbb{E}_{a_{t+1} }[-\text{log}~\pi_{\vect{\theta}}(a_{t+1}|s_{t+1})]\big]
\end{aligned}
\end{equation}
where  $\alpha > 0$ is a hyperparameter to trade-off between maximizing rewards and maximizing entropy. Adding the entropy bonus during environment interaction requires computing the expectation over successor states, which is challenging in model-free setting. Instead, an entropy term is augmented to the definition of the $Q$ and $V$ functions in SAC, giving rise to the soft $Q$ and soft $V$ functions which can be learned by a modified Bellman backup operator. Specifically, the soft $V$ function in SAC is defined as, 
\begin{equation}
    V_{\vect{\phi}}(s_t) = \mathbb{E}_{a_{t}\sim \pi }[Q_{\vect{\psi}}(s_t,a_t)-\alpha\text{log}~\pi_{\vect{\theta}}(a_t|s_{t})],
\end{equation}
where $Q_{\vect{\psi}}(s_t,a_t)$ is the soft $Q$ function,
\begin{equation}
    Q_{\vect{\psi}}(s_t,a_t) = \mathcal{R}(s_t,a_t) + \gamma \mathbb{E}_{s_{t+1}\sim \mathcal{P}}[V_{\vect{\phi}}(s_{t+1})].
\end{equation}
The parameters of both the soft $Q$ and $V$ functions can be learned by minimizing the mean squared Bellman error (MSBE) whereby the targets $\hat{Q}(s_t,a_t)$ and $\hat{V}(s_t)$ are formed based on target networks whose weights are periodically updated to match the weights of the current $Q_{\vect{\psi}}$ and $V_{\vect{\phi}}$ functions. Finally, the policy parameters are learned by maximizing the following objective function using stochastic gradient ascent and mini-batches sampled from the replay buffer $\mathcal{D}$,
\begin{equation}
    \mathcal{O}^\text{SAC}(\vect{\theta}) =\mathbb{E}_{s_t \sim \mathcal{D}}[Q_{\vect{\psi}}(s_t,\pi_{\vect{\theta}}(a_t|s_{t}))-\alpha \text{log}~\pi_{\vect{\theta}}(a_t|s_{t})].
\end{equation}

To enforce constraints in SAC, we train a parameterized policy $\pi_{\vect{\theta}}(a_t|s_t)$, a soft reward $Q$ function, $Q_{\vect{\psi}_0}$, and $K$ soft cost $Q$ functions, $Q_{\vect{\psi}_k}, k \in \{ 1,\cdots,K\}$, as follows. The policy parameters $\vect{\theta}$ are learned by optimizing an objective function in which the composition of the state-action value function with the actor policy  and the entropy of the policy are maximized, while the cost critics are minimized,
\begin{equation} \label{policy:obj}
\begin{aligned}
    \mathcal{O}^{\text{CSAC}}(\vect{\theta})= \mathbb{E}\Big[& Q_{\vect{\psi}_0}(s_{t},\pi_{\vect{\theta}}(a_t|s_{t}))-\alpha \text{log}~\pi_{\vect{\theta}}(a_t|s_t) \\
& -\sum_{k=1}^K \lambda_k Q_{\vect{\psi}_k}(s_{t},\pi_{\vect{\theta}}(a_t|s_{t})) \Big].
\end{aligned}
\end{equation}
To reduce overestimation bias induced by function approximation \cite{fujimoto2018addressing}, we train two reward critics, and take the minimum of the two reward critics in the policy improvement step \cite{fujimoto2018addressing}. Furthermore, we train two of each cost critic, and take the maximum of the two cost critics to reduce underestimation bias. %Overestimation bias is especially problematic due to its propagation through Bellman backups. To see how overestimation arises, consider the update rule in Q-learning (or critic updates in general) which estimates the target values  based on the estimation of $\mathbb{E}_\epsilon [ \underset{a} max~ \big(Q(s_{t+1},a)+ \epsilon \big)] \geq \underset{a} max~ Q(s_{t+1},a)+ \mathbb{E}_\epsilon [\epsilon]$, where $\epsilon$ is a function approximation error. Even if  $\epsilon$ has zero-mean, the target Q-values will be overestimated. Taking the minimum of two reward critics helps reduce the overestimation bias.
The reward (cost) critic is learned by minimizing the MSBE where the target is formed by taking the minimum (maximum) of the two target reward critics to promote  regression stability,  
\begin{equation} \label{q:obj}
    \mathcal{O}^Q(\vect{\psi}_{i})= \mathbb{E}\Bigg[ \bigg( Q_{\vect{\psi}_i}(s_t,a_t) - Q^\text{target}_i
     \bigg)^2
    \Bigg],
\end{equation}
where $Q^\text{target}_0 = \mathcal{R}(s_t,a_t) + \gamma \Big( \underset{i}{\text{min}}~ Q_{\bar{\vect{\psi}}_0}(s_{t+1},\pi_{\vect{\theta}}(a_{t+1}|s_{t+1}))$ $- \alpha \text{log}~\pi_{\vect{\theta}}(a_{t+1}|s_{t+1}) \Big)$, and  $Q^\text{target}_k = \mathcal{C}(s_t) + \gamma \Big( \underset{i}{\text{max}}~$ $ Q_{\bar{\vect{\psi}}_k}(s_{t+1},\pi_{\vect{\theta}}(a_{t+1}|s_{t+1}))$ $- \alpha \text{log}~\pi_{\vect{\theta}}(a_{t+1}|s_{t+1}) \Big)$. Here $\bar{\vect{\psi}}_i$ refers to the parameters of the target network.
\end{comment}

\begin{comment}
\begin{algorithm} 
 \SetKwInOut{Input}{Input}
    \LinesNotNumbered
    \textbf{Initialize:} DNN parameters DNN of the policy $\pi_{\vect{\theta_\pi}}$, two reward Q-functions  $Q^R_{\vect{\theta_{1R}}}$, $Q^R_{\vect{\theta_{2R}}}$, and $K$ cost Q-functions $Q^C_{\vect{\theta_{kC}}}$, replay buffer $\mathcal{T}_B$, $\delta_k,\forall k$\\  
\For{$k=0,1, \cdots$ }
{
\For{$t=0,1, \cdots$, T}
{
Observe initial state $s_t$ \\
Sample action $a_t \sim \pi_{\vect{\theta_\pi}}(a_t|s_t)$\\
Take action $a_t$\\
Receive reward $\mathcal{R}(s_t,a_t)$, $K$ costs $\mathcal{C}_k(s_t,a_t)$, and new state $s_{t+1}$\\
Store transition $(s_t,a_t,\mathcal{R}(s_t,a_t),\mathcal{C}_{k,\forall k}(s_t,a_t),s_{t+1})$ in $\mathcal{T}_B$\\
}
\For{each gradient step}
{
Randomly sample a batch of transitions from $\mathcal{T}_B$\\
Update reward Q-function parameters  $\vect{\theta_{1R}}, \vect{\theta_{2R}}$ by gradient descent on \eqref{q:obj} \\
Update cost Q-function parameters  $\vect{\theta_{kC}},\forall k$ by gradient descent on \eqref{c:obj} \\
Update policy parameters $\vect{\theta_\pi}$ by gradient ascent on \eqref{policy:obj} \\
Update target networks $Q^{R^\prime}_{\vect{\theta_{1R}}}$, $Q^{R^\prime}_{\vect{\theta_{2R}}}$, and $Q^{C^\prime}_{\vect{\theta_{kC}}}, \forall k$ through polyak averaging: $\vect{\theta}^\prime \leftarrow \tau \vect{\theta} + (1-\tau)\vect{\theta}^\prime$\\
Update dual variables, $\forall k$: $\eta_k \leftarrow \text{max} \{0, \eta_k + \delta_k (\mathbb{E}_{s_t \sim \mathcal{T}_B }[Q^C_{\vect{\theta_{kC}}}(s_t,\pi(s_t))] - E_k) \}$\\
}
}
    \caption{Online Soft Actor Critic CDRL} \label{alg:Alg3}
\end{algorithm}
\end{comment}




 \begin{comment}
\section{Chance Constrained RL with a Stochastic Safety Layer}

In this subsection, we propose an alternative formulation to learn safe policies with model-free RL methods. Instead of having one chance constraint  that depicts the probability of a joint event over the operating horizon $T$, we propose an alternative formulation whereby $T$ disjoint chance constraints are imposed,
\begin{equation} \label{eq:ccrl3}
\begin{aligned}
&\underset{\pi}{\text{max}}~\mathbb{E}_{a_t \sim \pi, s_{t+1} \sim P, s_0 \sim \beta} \Big[ \sum_{t=0}^{T-1} \gamma^t \mathcal{R}(s_t,a_t) \Big] \\
& \text{Pr}\Big[  s_{t+1} \in \mathcal{S}_{\text{safe}} \Big] \geq 1-K\delta,  t \in \{0,\cdots,T-1\}.
\end{aligned}
\end{equation}
Here it is assumed that $s_0 \in \mathcal{S}_{\text{safe}}$, $\forall s_0 \sim \beta$. Because the chance constraints are disjoint over the operating horizon $T$, learning a safe policy reduces to learning safe state-wise actions. Recall that \eqref{eq:ccrl3} can be alternatively expressed (with extra conservatism) as $K$ constraint functions of the state, 
\begin{equation} \label{eq:ccrl4}
\begin{aligned}
&\underset{\pi}{\text{max}}~\mathbb{E}_{a_t \sim \pi, s_{t+1} \sim P, s_0 \sim \beta} \Big[ \sum_{t=0}^{T-1} \gamma^t \mathcal{R}(s_t,a_t) \Big] \\
& \text{Pr}\Big[  \mathcal{T}_k(s_{t+1}) \geq 0 \Big] \leq \delta,  k \in \{1,\cdots,K\}.
\end{aligned}
\end{equation}

Intuitively, if we can predict whether an action $a_t$ at time step $t$ will drive the system out of the safe region, then we can rectify the action before it is executed to avoid the violation. This rectification can be performed by transporting the state-dependent action distribution $\pi_{\vect{\theta}}(a_t|s_t)$ to another distribution $\hat{\pi}_{\vect{\theta}}(a_t|s_t)$ that ensures an action sampled $a_t\sim \hat{\pi}_{\vect{\theta}}(a_t|s_t)$ will keep the system in the safety region with high probability. Notice that our proposed method is a generalization of the safety layer proposed \cite{dalal2018safe} which only ensures that the \textit{\textbf{mean}} of the policy is safe.

Mathematically, our proposed \textit{stochastic safety layer} minimizes the squared Wasserstein distance $||W_2(\pi, \hat{\pi})||^2$ between $\pi_{\vect{\theta}}(a_t|s_t) $ %$\sim \mathcal{N}(\vect{\mu}_{\vect{\theta}}(s_t),\vect{C}_{\vect{\theta}}(s_t))$ 
(which is considered fixed for the purpose of safety projection) and the new safe distribution $\hat{\pi}_{\vect{\theta}}(a_t|s_t)$ %$\sim \mathcal{N}(\hat{\vect{\mu}},\hat{\sigma}^2\mathbb{I})$ 
subject to a lookahead chance constraint at each time step $t$ that ensures the policies probability of violating constraint $k$ is less than or equal to $\delta$, 

\begin{equation} \label{eq:ccrl5}
\begin{aligned}
&\underset{}{\text{min}}~||W_2(\pi, \hat{\pi})||^2 \\
& \text{Pr}\Big[ \mathcal{T}_k( s_{t+1} ) \geq 0 \Big] \leq \delta,  k \in \{1,\cdots,K\}.
\end{aligned}
\end{equation}
Specifically, at each time step $t$ during the agent's environment interaction, the agent's policy is projected to the safe region by solving  \eqref{eq:ccrl5}. To update policy parameters $\vect{\theta}$ with policy gradient methods during training, we need to backpropagate the errors through the optimization problem \eqref{eq:ccrl5}, which requires problem \eqref{eq:ccrl5} to be differentiable with respect to $\vect{\theta}$. For mathematical tractability, in this work we focus on 
a setup that allows us to derive the algebraic solution for \eqref{eq:ccrl5} which can be then coded as a differentiable layer with few lines of code. To this end, we consider circular Gaussian policies of the form $\pi_{\vect{\theta}}(a_t|s_t) \sim \mathcal{N}(\vect{\mu}_{\vect{\theta}}(s_t),\vect{C}_{\vect{\theta}}(s_t))$, i.e., the mean $\vect{\mu}_{\vect{\theta}}(s_t)$  and covariance matrix $\vect{C}_{\vect{\theta}}(s_t) =\mathbb{I}* \sigma^2_{\vect{\theta}}(s_t)$ at a state $s_t$ are modeled by  a multi-headed parameterized DNN with parameters $\vect{\theta}$, where $\mathbb{I}$ is the identity matrix. Similarly,  $\hat{\pi}_{\vect{\theta}}(a_t|s_t) \sim \mathcal{N}(\hat{\vect{\mu}},\hat{\sigma}^2\mathbb{I})$. Furthermore, we consider that a locally linear cost-dynamics model which predicts the cost incurred at the next state $s_{t+1}$ given the current state-action pair $(s_t,a_t)$ is available. Such cost-dynamics model can be learned offline before the agent is trained as in \cite{dalal2018safe}. For instance, a DNN $\mathcal{G
}: \mathcal{S} \times \mathcal{A} \rightarrow \mathbb{R}^K$ can be trained to predict the $k$-th cost of the state at the next time state $\mathcal{T}_k(s_{t+1})$ (output) given current $(s_t,a_t)$ features (inputs) based on data set of input-output pairs $\mathcal{D}_c = \{(s_t^i,a_t^i), \mathcal{T}_k(s_{t+1}^i)\}_{i=1}^N$. Once $\mathcal{G}$ is learned, the locally linear model $\hat{\mathcal{T}}_k(s_{t},a_t)= \vect{A}^k_t s_t + \vect{B}^k_t a_t \approx \mathcal{T}_k(s_{t+1})$, can be derived by performing a first order Taylor approximation of $\mathcal{G}$ to compute the vectors $(\vect{A}^k_t,\vect{B}^k_t)$. Lastly, we assume that only one  constraint $k$ is active at a time. % 
Based on this setup, the squared Wasserstein distance $||W_2(\pi, \hat{\pi})||^2$ can be computed in closed-form as $||W_2(\pi, \hat{\pi})||^2 = ||\vect{\mu}_{\vect{\theta}}(s_t) - \hat{\vect{\mu}} ||_2^2 + 2 ({\sigma}_{\vect{\theta}}(s_t)-\hat{\sigma})^2 $. %Because a linear transformation of a gaussian random variable is also gaussian, $\mathcal{T}_k(s_{t+1})$ is also gaussian distributed. 
Additionally, a Chernoff bound is leveraged  \cite{khairy2022multifidelity} to upper bound $\text{Pr}\Big[ \mathcal{T}_k( s_{t+1} ) \geq 0 \Big] \leq \text{exp}\big( -\frac{(\mathbb{E}[\mathcal{T}_k( s_{t+1} )])^2}{2\text{Var}[\mathcal{T}_k( s_{t+1} )]} \big) $, where $\mathbb{E}[\mathcal{T}_k( s_{t+1} )]=\vect{A}^k_t s_t + \vect{B}^k_t \hat{\vect{\mu}} $ and $\text{Var}[\mathcal{T}_k( s_{t+1} )]= \vect{B}^k_t(\vect{B}^k_t)^T \hat{\sigma}^2 $. Hence by linear approximation of the cost-dynamics and using a Chernoff bound \eqref{eq:ccrl5} becomes, 
\begin{equation} \label{eq:ccrl6}
\begin{aligned}
&\underset{\hat{\vect{\mu}},\hat{\sigma}}{\text{min}}~||\vect{\mu}_{\vect{\theta}}(s_t) - \hat{\vect{\mu}} ||_2^2 + 2 ({\sigma}_{\vect{\theta}}(s_t)-\hat{\sigma})^2  \\
&  {(\vect{A}^k_t s_t + \vect{B}^k_t \hat{\vect{\mu}})^2}  \geq \hat{\sigma}^2 (-2\vect{B}^k_t(\vect{B}^k_t)^T  \text{log}\delta).
\end{aligned}
\end{equation}
Notice that the objective function in \eqref{eq:ccrl6} is a quadratic convex function in the decision variables $(\hat{\vect{\mu}},\hat{\sigma})$, however, the constraints are non-convex. Nevertheless, each non-convex constraint is a union of two disjoint convex sets (because $\hat{\sigma}\geq0$), ${(\vect{A}^k_t s_t + \vect{B}^k_t \hat{\vect{\mu}})}  \geq \hat{\sigma} w_t^k $ and ${(\vect{A}^k_t s_t + \vect{B}^k_t \hat{\vect{\mu}})}  \leq -\hat{\sigma} w_t^k $, where $w_t^k = \sqrt{(-2\vect{B}^k_t(\vect{B}^k_t)^T  \text{log}\delta)}$. Hence, we can solve the optimization problem twice, once on each local domain to find two local solutions, and lastly pick the globally optimal solution. On each local domain, we have a convex optimization problem that can be analytically solved by deriving the KKT conditions.  First, we form the Lagrangian function for \eqref{eq:ccrl6},
\begin{equation} \label{eq:lagrange}
\begin{aligned}
L(\hat{\vect{\mu}},\hat{\sigma},\lambda) &= ||\vect{\mu}_{\vect{\theta}}(s_t) - \hat{\vect{\mu}} ||_2^2 + 2 ({\sigma}_{\vect{\theta}}(s_t)-\hat{\sigma})^2 \\
&+ \lambda_k \Big(\mp (\vect{A}^k_t s_t + \vect{B}^k_t \hat{\vect{\mu}}) + \hat{\sigma} w_t^k \Big).
\end{aligned}
\end{equation}
The stationary condition at $(\hat{\vect{\mu}}^*,\hat{\sigma}^*, \lambda_k^*)$ implies that, 
\begin{equation} \label{eq:stationarity}
\begin{aligned}
    \nabla_{\hat{\vect{\mu}}}L &= -2 (\vect{\mu}_{\vect{\theta}}(s_t) - \hat{\vect{\mu}} ) \mp \lambda_k\vect{B}^k_t = 0 \\ &\implies \hat{\vect{\mu}}  =  \vect{\mu}_{\vect{\theta}}(s_t)  \pm \frac{
    1}{2}\lambda_k\vect{B}^k_t,
    \\
     \nabla_{\hat{\sigma}}L &= -4 ({\sigma}_{\vect{\theta}}(s_t)-\hat{\sigma}) + \lambda_kw_t^k = 0
     \\
     &\implies  \hat{\sigma} = {\sigma}_{\vect{\theta}}(s_t) - \frac{
    1}{4}\lambda_kw_t^k
\end{aligned}
\end{equation}
The complimentary slackness condition states that $\lambda_k \Big(\mp (\vect{A}^k_t s_t + \vect{B}^k_t \hat{\vect{\mu}}) + \hat{\sigma} w_t^k \Big) = 0, \forall k$. Since one constraint is active at a time, $\lambda_i > 0$ for $i=k$ and $\lambda_i = 0, \forall k \in \{0,\cdots, k-1,k+1, \cdots, K\}$, which implies that $\Big(\mp (\vect{A}^k_t s_t + \vect{B}^k_t \hat{\vect{\mu}}) + \hat{\sigma} w_t^k \Big)=0$. By plugging \eqref{eq:stationarity} into the active constraint and solving for $\lambda_k$,

%
%\begin{equation}
%\begin{aligned}
%\mp \vect{A}^k_t s_t \mp \vect{B}^k_t (\vect{\mu}_{\vect{\theta}}(s_t)  \pm \frac{
%    1}{2}\lambda_k\vect{B}^k_t)  + ({\sigma}_{\vect{\theta}}(s_t) - \frac{
%    1}{4}\lambda_kw_t^k) w_t^k = 0 
%\end{aligned}
%\end{equation}
%and solve for $\lambda_k$, 

\begin{equation}
\begin{aligned}
\lambda_k= \Bigg[\frac{\mp \vect{A}^k_t s_t \mp \vect{B}^k_t\vect{\mu}_{\vect{\theta}}(s_t)  
  + w_t^k{\sigma}_{\vect{\theta}}(s_t)}{\frac{
    1}{4}(w_t^k)^2 \pm \frac{
    1}{2}\vect{B}^k_t\vect{B}^k_t} \Bigg]^+,
\end{aligned}
\end{equation}
where $[~]^+$ denotes the non-negative part, which ensures dual feasibility, i.e., $\lambda_k \geq 0, \forall k$.

\end{comment}



%Reinforcement learning~(RL) is concerned with how agents should take actions in an environment to obtain the maximal reward from the environment for specific goals. In recent years, RL has become the foundation of many breakthroughs in artificial intelligence, such as AlphaGo [cite] and AlphaZero [cite]. Model-free RL has been a research focus for many scientific applications, given its flexibility and applicability to complex real-world environments [cite].

% In this work, we follow the regime of the first type and derive a modified reward function from a chance-constrained reinforcement learning problem.
 
% A constrained Markov Decision Process~(cMDP) describes the safety-constrained reinforcement learning problem. A cMDP has additional constraint functions space, $\mathcal{C}$, and constraint bounds, $b$. 
% 
% The constraints are known a priori. \cite{brunkeSafeLearningRobotics2021}. Our work formulates the problem as a constrained Markov Decision Process.

%While $\hat{p}_s(\pi)$ can be easily estimated based on collected experience, the gradient of the safe probability with respect to the policy parameters $\vect{\theta}$, $\nabla_{\vect{\theta}} p_s(\pi)$ is discontinuous and non-differentiable. 

%there is no analytical solution for the joint probability or its gradient. In addition, the chance constraint depends not only on $\pi$, but also on the system's dynamics $P$ and the initial state distribution $\beta$ which are unknown to the agent.

%Optimization is performed over three time-scales, on the fastest time scale, the state-value function is updated by minimizing \eqref{mse:V}, then the policy is updated by maximizing \eqref{ppo} on the intermediate time-scale, and finally, the Lagrangian multipliers are updated on the slowest time-scale by minimizing \eqref{lag:loss}. Optimization time-scales are controlled by choosing the maximum learning rate of the stochastic gradient optimizer used, e.g., adaptive moment estimation (ADAM) \cite{kingma2014adam}, as well as the number of gradient steps performed at the end of each training epoch. %The full algorithmic procedure for training the CDRL agent is outlined in Algorithm $1$.
